# Supplementary material for: DeCOM: Decomposed Policy for Constrained Cooperative Multi-Agent Reinforcement Learning
Source: arXiv:2111.05670 source file (2021-11-10)
Supplement: Supplementary file 1 [file appendix_alg.tex]

\subsection{DeCOM Algorithm and Convergence Analysis}\label{decom}

\subsubsection{Convergence Analysis}\label{decom:convergence}
In DeCOM algorithm, network parameters are actually governed by following stochastic update recursions respectively (we assume $M=1$ here for simplicity, while it is intuitive to extend into $M>1$):
\begin{equation}
    \begin{aligned}
    \eta_{k+1} & = \eta_k + \alpha_k^{\eta}\cdot\bigg(r+\gamma Q^{\eta'_{k}}(s', \boldsymbol{a}')-Q^{\eta_{k}}(s, \boldsymbol{a})\bigg)\frac{\partial Q^{\eta}(s, \boldsymbol{a})}{\partial\eta}\\
    \zeta_{k+1} & = \zeta_k + \alpha_k^{\zeta}\cdot\bigg(c+\gamma Q^{\zeta'_{k}}(s', \boldsymbol{a}')-Q^{\zeta_{k}}(s, \boldsymbol{a})\bigg)\frac{\partial Q^{\zeta}(s, \boldsymbol{a})}{\partial\zeta}\\
    \boldsymbol{\theta}_{k+1} & = \boldsymbol{\theta}_k + \alpha_k^{\theta}\cdot\frac{\partial J^R(f_{\boldsymbol{\theta}}, \boldsymbol{g}_{\boldsymbol{\phi}})}{\partial\boldsymbol{\theta}}\\
    \boldsymbol{\phi}_{k+1} & = \boldsymbol{\phi}_k - \alpha_k^{\phi}\cdot\frac{\partial \mathcal{L}(\boldsymbol{\theta}, \boldsymbol{\phi})}{\partial\boldsymbol{\phi}},
    \end{aligned}
\end{equation}
where $\alpha_k^{*}$ is the learning rate for parameter $*$. The convergence of $(\eta_k, \zeta_k, \boldsymbol{\theta}_k, \boldsymbol{\phi}_k)$ to stationary points can be analyzed under multi-timescale stochastic approximation processes \cite{borkar2009stochastic} framework, within which the schedule of learning rate is of great importance. We set following schedule for the learning rate \footnote{Similar learning rate schedules have been shown in \cite{tessler2018reward, pmlr-v97-chandak19a}.}:

\textbf{Learning Rate Schedule.} The learning rate $\alpha_k^{\eta}$, $\alpha_k^{\zeta}$, $\alpha_k^{\theta}$, $\alpha_k^{\phi}$ satisfy:
\begin{gather}
    \sum_k \alpha_k^{\eta} = \infty, \sum_k \alpha_k^{\zeta} = \infty, \sum_k \alpha_k^{\theta} = \infty, \sum_k \alpha_k^{\phi} = \infty,\nonumber\\
    \sum_k (\alpha_k^{\eta})^2 < \infty, \sum_k (\alpha_k^{\zeta})^2 < \infty, \sum_k (\alpha_k^{\theta})^2 < \infty, \sum_k (\alpha_k^{\phi})^2 < \infty,\nonumber\\
    \text{As }\,k\rightarrow\infty, \frac{\alpha_k^{\theta}}{\alpha_k^{\phi}}\rightarrow 0, \frac{\alpha_k^{\phi}}{\alpha_k^{\eta}}\rightarrow 0, 
    \frac{\alpha_k^{\phi}}{\alpha_k^{\zeta}}\rightarrow 0. \label{lr:large_small}
\end{gather}
Condition (\ref{lr:large_small}) requires that, the reward critic and cost critic updates on the fastest timescale and the base policy $f_{\boldsymbol{\theta}}$ updates on the slowest. Under this difference timescale setting, the subsequent convergence analysis becomes common and standard, with the multi-timescale stochastic approximation processes \cite{borkar2009stochastic} framework.
